# Supplementary material for: Maat: Performance Metric Anomaly Anticipation for Cloud Services with Conditional Diffusion
Source: arXiv:2308.07676 source file (2023-08-15)
Supplement: Supplementary file 1 [file appendix.tex]

\section{Compared Methods}
\subsection{Real-time Anomaly Detectors}\label{sec:appendix:detect}
\begin{itemize}
    \item Dount~\cite{dount} is an unsupervised anomaly detection algorithm for univariate metrics based on Variational Autoencoder (VAE). It compares the reconstructed metrics and the really observed metrics and alerts anomalies when obtaining a large reconstruction loss.
    \item SR-CNN~\cite{srcnn} applies residual spectrum (SR) from the visual saliency detection domain to time series anomaly detection. The SR model generates pseudo labels to train the subsequent convolutional neural network, which will output a binary result to indicate anomalies.
    \item Adsketch~\cite{adsketch} is a recently proposed method that adaptively detects performance anomalies based on pattern sketching. It is semi-supervised in a sense as it requires anomaly-free inputs to extract normal patterns. If the current metric patterns are not similar to previous patterns, an alarm will be triggered.
    \item Telemanom~\cite{telemanom} combines long-short-term-memory (LSTM) with an auto-thresholding algorithm. The trained LSTM first predicts the next-time metric, and if the prediction error is larger than the automatically decided threshold, Telemanom will report an anomaly.
    \item LSTM-VAE~\cite{lstm-vae} also works by reconstructing subsequences of metrics, similar to Dount. It combines LSTM with VAE and can handle multivariate time series.
    \item MTAD-GAT~\cite{mtad} combines both prediction-based approaches (e.g., Telemanom) and reconstruction-based approaches (e.g., Dount). It considers every single metric as a feature and then uses two parallel graph attention network (GAT) layers to learn the temporal and cross-metric dependencies. The two models will jointly output an inference score as the basis of anomaly detection.
    \item DAGMM~\cite{dagmm} combines a deep autoencoder and a Gaussian Mixture Model to estimate the anomaly score of each to-be-detected metric subsequence.
    \item OmniAnomaly~\cite{OmniAnomaly} is a stochastic recurrent neural network for multivariate time series anomaly detection based on VAE. It aims to learn potential representations to capture normal patterns of metrics while considering time dependencies and stochasticity.
\end{itemize}

\subsection{Time Series Forecasting Baselines}\label{sec:appendix:pred}
\begin{itemize}
    \item DeepVAR~\cite{DeepVAR} is a time series distribution forecasting model by combining LSTM with the Gaussian Copula process. It allows modeling time-varying correlations between high-dimensional time series.
    \item GRU-MAF and Transformer-MAF~\cite{condFlow} represents the data distribution by a conditioned normalizing flow, i.e., masked autoregressive flow (MAF)~\cite{MAF}, combined with an autoregressive deep learning model. We follow the original paper~\cite{condFlow} to set the model as GRU and Transformer, respectively.
\end{itemize}
